# Supplementary material for: nach0-pc: Multi-task Language Model with Molecular Point Cloud Encoder
Source: arXiv:2410.09240 source file (2024-10-11)
Supplement: Supplementary file 1 [file datasets.tex]

\begin{tabular}{|c|c|c|c|}
\hline
Dataset & Split source & Statistics & \# Tokens\\ \hline
MOSES & \cite{polykovskiy2020moses} & 1.5m mols, 1 conf./mol. & 663M \\ \hline
ZINC \cite{irwin2005zinc} & \cite{igashov2022difflinker} & 400k mols, 1 conf./mol. & 27M \\ \hline
GEOM-DRUGS \cite{axelrod2022geom} & \cite{igashov2022difflinker} & 300k mols, $\sim$50 conf./mol. & 4B \\ \hline
\end{tabular}
